# Supplementary material for: Stochastic Modelling of Symmetric Positive Definite Material Tensors
Source: arXiv:2109.07962 source file (2024-02-09)
Supplement: Supplementary file 1 [file appendix.tex]

% !TEX root = ../paper_tensors.tex
% !TEX encoding = UTF-8 Unicode

%\appendix

\newcommand{\Croneone}{\meansymb{H}_r^{11}}
\newcommand{\Cronetwo}{\meansymb{H}_r^{12}}
\newcommand{\Crtwoone}{\meansymb{H}_r^{21}}
\newcommand{\Crtwotwo}{\meansymb{H}_r^{22}}

\newcommand{\Crsoneone}{\meansymb{H}_{rs}^{11}}

\newcommand{\Roneone}{R_{11}(\event_r)}
\newcommand{\Ronetwo}{R_{12}(\event_r)}
\newcommand{\Rtwoone}{R_{21}(\event_r)}
\newcommand{\Rtwotwo}{R_{22}(\event_r)}

\section{Euclidean mean in 2D}\label{App:derivation}

The Euclidean mean---connected to the Euclidean metric---is one of the most commonly used measures to determine the expectation of a real-valued symmetric random tensor. 
% in $\SymSecRankSpace$. 
For instance, the arithmetic mean is suitable in determining the mean of a random diagonal matrix, $\symdiag_s(\event_s)\in \SymSecRankSpace$ from \feq{Eq:rndscl}---the case of random scaling only. 
However, as we know that the Euclidean distance does not satisfy all the desired properties of a metric listed in \fsec{Sec:Problem}, the metrics like $\vartheta_G$ and $\vartheta_L$ are hence considered to be more appropriate. 
We also come across the other downside of using arithmetic mean when rotational uncertainty is incorporated into the modelling scenario, such as the random tensor $\symtensor_r(\event_r)\in \SymSecRankSpace$ in \feq{Eq:stomodrot}. That is, the Euclidean mean of $\symtensor_r(\event_r)$
does not converge to the corresponding reference tensor $\meanH_r$, in other words, the Euclidean mean gets distorted. 
Such a result is shown for the 2D case, $d=2$.
% However, as we know that the Euclidean distance does not satisfy all the desired properties of a metric listed in \fsec{Sec:Problem}. 

Let us re-represent the random rotation matrix $\rotmat(\event_r)\in\text{SO}(2)$ given in \feq{Eq:Rmatrix} as
\begin{equation}\label{Eq:A1}
\rotmat(\event_r) =
\begin{bmatrix}
\Roneone & \Ronetwo  \\ \Rtwoone & \Rtwotwo
\end{bmatrix},
\end{equation}
and similarly, the reference tensor $\meanH_r\in\SymSecRankSpacetwoD$ in \feq{Eq:meanrot} as
\begin{equation}\label{Eq:A2}
\meanH_r =
\begin{bmatrix}
\Croneone & \Cronetwo  \\ \Crtwoone & \Crtwotwo
\end{bmatrix}.
\end{equation}
Consequently, the stochastic tensor $\symtensor_r(\event_r)\in \SymSecRankSpacetwoD$---with random orientations only---may also be rewritten in the form:
\begin{equation}
\symtensor_r(\event_r) =
\rotmat(\event_r) \meanH_r \rotmat(\event_r)^T =
\begin{bmatrix}
H_r^{11}(\event_r) & H_r^{12}(\event_r)  \\ H_r^{21}(\event_r) & H_r^{22}(\event_r)
\end{bmatrix}.
\end{equation}
From \feq{Eq:stomodrot}, the Euclidean mean of the above random tensor takes the form:
\begin{equation}\label{Eq:stomodrot1}
\mathbb{E}[\symtensor_r(\event_r)]
= \mathbb{E}[\rotmat(\event_r) \meanH_r \rotmat(\event_r)^T]
= \begin{bmatrix}
\mathbb{E}[H_r^{11}(\event_r)] & \mathbb{E}[H_r^{12}(\event_r)]  \\ \mathbb{E}[H_r^{21}(\event_r)] & \mathbb{E}[H_r^{22}(\event_r)]
\end{bmatrix}.
\end{equation}
To determine the Euclidean mean of the three upper triangular components in the above matrix,
% $\mathbb{E}[\randrot^{11}(\event_r)]$, $\mathbb{E}[\randrot^{12}(\event_r)]$ and $\mathbb{E}[\randrot^{22}(\event_r)]$.
let us substitute the \feqs{Eq:A1}{Eq:A2} in \feq{Eq:stomodrot1}. Accordingly, one can expand the element $\mathbb{E}[H_r^{11}(\event_r)]$ as
%\begin{equation}
\begin{multline}\label{Eq:A5}
\mathbb{E}[H_r^{11}(\event_r)] = \mathbb{E}[\Roneone^2]\Croneone+\mathbb{E}[\Roneone\Ronetwo]\Crtwoone + \\ \mathbb{E}[\Ronetwo\Roneone]\Cronetwo +\mathbb{E}[\Ronetwo^2]\Crtwotwo, 
\end{multline}
%\end{equation}
in which 
%\begin{equation}
\begin{align}
\mathbb{E}[\Roneone^2] &= \mathbb{E}[\cos^2(\rotangle(\event_r))] = \mathbb{E}\left[ \frac{1+\cos 2\rotangle(\event_r)}{2}\right],  \\
\mathbb{E}[\Roneone\Ronetwo] &=  -\mathbb{E}[\sin(\rotangle(\event_r))\cos(\rotangle(\event_r))] =  -\mathbb{E}\left[ \frac{\sin 2\rotangle(\event_r)}{2}\right], \\
\mathbb{E}[\Ronetwo^2] &= \mathbb{E}[\sin^2(\rotangle(\event_r))] = \mathbb{E}\left[ \frac{1-\cos 2\rotangle(\event_r)}{2}\right]. 
\end{align}
%\end{equation}
%\begin{equation}
%\begin{split}
%\mathbb{E}[\Roneone\Ronetwo] =  -\mathbb{E}[\sin(\rotangle(\event_r))\cos(\rotangle(\event_r))] =  -\mathbb{E}\left[ \frac{\sin 2\rotangle(\event_r)}{2}\right].
%\end{split}
%\end{equation}
%and
%\begin{equation}
%\begin{split}
%\mathbb{E}[\Ronetwo^2] = \mathbb{E}[\sin^2(\rotangle(\event_r))] = \mathbb{E}\left[ \frac{1-\cos 2\rotangle(\event_r)}{2}\right] 
%\end{split}
%\end{equation}
Given the mean direction $\circmeananly=0$ of the symmetric circular variable $\rotangle(\event_r)$, the properties of trigonometric moments \cite{mardia_directional_2000,jammalamadaka_topics_2001}, such as
\begin{align}\label{Eq:TrigProp}
	\mathbb{E}[\sin2(\rotangle(\event_r))] &= 0, \\ \nonumber
	\mathbb{E}[\cos2(\rotangle(\event_r))] &= \rho_2,
\end{align}
%$\mathbb{E}[\sin2(\rotangle(\event_r))] = 0$ and 
%$\mathbb{E}[\cos2(\rotangle(\event_r))] = \rho_2,$
reduce the
above equations to:
\begin{align}
	\mathbb{E}[\Roneone^2] &= \frac{1}{2}+\frac{\rho_2}{2}, \label{Eq:A9} \\
	\mathbb{E}[\Roneone\Ronetwo] &= 0, \label{Eq:A10} \\
	\mathbb{E}[\Ronetwo^2] &= \frac{1}{2}-\frac{\rho_2}{2}, \label{Eq:A11}
\end{align}
where $\rho_2\in[0,1]$ is the population circular variance of doubled random variable $2\rotangle(\event_r)$.
Therefore, by substituting \feeqs{Eq:A9}{Eq:A11} into \feq{Eq:A5}, the term $\mathbb{E}[H_r^{11}(\event_r)]$ transforms to
\begin{equation}\label{Eq:A13}
\mathbb{E}[H_r^{11}(\event_r)] = \frac{\Croneone+\Crtwotwo}{2} + \frac{\rho_2}{2}(\Croneone-\Crtwotwo).
\end{equation}
Similarly, the component $\mathbb{E}[H_r^{12}(\event_r)]$ is expressed in the form:
\begin{multline}\label{Eq:A14}
\mathbb{E}[H_r^{12}(\event_r)] = \mathbb{E}[\Rtwoone\Roneone]\Croneone+\mathbb{E}[\Rtwoone\Ronetwo]\Crtwoone\\+\mathbb{E}[\Rtwotwo\Roneone]\Cronetwo +\mathbb{E}[\Rtwotwo\Ronetwo]\Crtwotwo.
\end{multline}
%\end{equation}
Following the properties defined in \feq{Eq:TrigProp}, one may define the entities in the above equation as
\begin{align}
	\mathbb{E}[\Rtwoone\Roneone] &= \mathbb{E}[\sin(\rotangle(\event_r))\cos(\rotangle(\event_r))] = 0, \label{Eq:A15} \\
	\mathbb{E}[\Rtwoone\Ronetwo] &= -\mathbb{E}[\sin^2(\rotangle(\event_r))] = \frac{\rho_2}{2}-\frac{1}{2}, \\
	\mathbb{E}[\Rtwotwo\Roneone] &= \mathbb{E}[\cos^2(\rotangle(\event_r))] = \frac{1}{2}+\frac{\rho_2}{2}, \\
	\mathbb{E}[\Rtwotwo\Ronetwo] &= -\mathbb{E}[\sin(\rotangle(\event_r))\cos(\rotangle(\event_r))] = 0. \label{Eq:A18}
\end{align}
Inserting the \feeqs{Eq:A15}{Eq:A18} in \feq{Eq:A14}, we thus obtain:
\begin{equation}\label{Eq:A19}
	\mathbb{E}[H_r^{12}(\event_r)] = \Cronetwo\rho_2.
\end{equation}

%$$ {C}_r^{21}(\event_r) = \Roneone\Rtwoone\Croneone+\Roneone\Rtwotwo\Crtwoone+\Ronetwo\Rtwoone\Cronetwo+\Ronetwo\Rtwotwo\Crtwotwo $$

%\begin{equation}
%\begin{split}
%\mathbb{E}[\randrot^{21}(\event_r)] = \mathbb{E}[\Roneone\Rtwoone]\Croneone+\mathbb{E}[\Roneone\Rtwotwo]\Crtwoone\\ +\mathbb{E}[\Ronetwo\Rtwoone]\Cronetwo
%+\mathbb{E}[\Ronetwo\Rtwotwo]\Crtwotwo
%\end{split}
%\end{equation}
%
%\begin{equation}
%	\mathbb{E}[\randrot^{21}(\event_r)] = \Crtwoone\rho_2
%\end{equation}

%$$ {C}_r^{22}(\event_r) = \Rtwoone^2\Croneone+\Rtwoone\Rtwotwo\Crtwoone+\Rtwotwo\Rtwoone\Cronetwo+\Rtwotwo^2\Crtwotwo $$
%\begin{equation}

Furthermore, the term $\mathbb{E}[H_r^{22}(\event_r)]$ is expanded as
\begin{multline}\label{Eq:A20}
\mathbb{E}[H_r^{22}(\event_r)] = \mathbb{E}[\Rtwoone^2]\Croneone+\mathbb{E}[\Rtwoone\Rtwotwo]\Crtwoone \\ +\mathbb{E}[\Rtwotwo\Rtwoone]\Cronetwo  +\mathbb{E}[\Rtwotwo^2]\Crtwotwo,
\end{multline}	
%\end{equation}
whose components (in reference to \feq{Eq:TrigProp}) are given by
\begin{align}
\mathbb{E}[\Rtwoone^2] & = \mathbb{E}[\sin^2(\rotangle(\event_r))] = \frac{1}{2}-\frac{\rho_2}{2}, \label{Eq:A21} \\
\mathbb{E}[\Rtwoone\Rtwotwo] & = \mathbb{E}[\sin(\rotangle(\event_r))\cos(\rotangle(\event_r))] = 0, \\
\mathbb{E}[\Rtwotwo^2] & = \mathbb{E}[\cos^2(\rotangle(\event_r))] = \frac{1}{2}+\frac{\rho_2}{2}. \label{Eq:A23}
\end{align}
As a result of the substitution of \feeqs{Eq:A21}{Eq:A23} in \feq{Eq:A20} one obtains
\begin{equation}\label{Eq:A24}
\mathbb{E}[H_r^{22}(\event_r)] = \dfrac{\Croneone+\Crtwotwo}{2} + \dfrac{\rho_2}{2}(\Crtwotwo-\Croneone).
\end{equation}

Finally, the \feqss{Eq:A13}{Eq:A19}{Eq:A24} when substituted into \feq{Eq:stomodrot1} give the Euclidean mean of the stochastic tensor $\symtensor_r(\event_r)$ in the form:
\begin{equation}\label{Eq:A25}
\mathbb{E}[\symtensor_r(\event_r)] =
\begin{bmatrix}
 \begin{multlined}
 \dfrac{\Croneone+\Crtwotwo}{2} + \vspace{-0.5cm}\\
 \dfrac{\rho_2}{2}(\Croneone-\Crtwotwo)
 \end{multlined} 
 & (\Cronetwo)\rho_2  \\ (\Cronetwo)\rho_2 & 
 \begin{multlined}
 \dfrac{\Croneone+\Crtwotwo}{2} + \vspace{-0.5cm}\\ \dfrac{\rho_2}{2}(\Crtwotwo-\Croneone)
 \end{multlined}
\end{bmatrix}.
\end{equation}
It turns out that the spectral decomposition of the above matrix can be written as
\begin{equation}\label{Eq:A26}
\mathbb{E}[\symtensor_r(\event_r)] = \meaneigvect_r  \meansymb{\symdiag}_r^{'} \meaneigvect_r^T = \meanH_r^{'},
\end{equation}
where $\meansymb{\symdiag}_r^{'}\in\mathbb{R}^{2\times 2}$ is the deformed diagonal matrix of real-valued eigenvalues (here $\meansymb{\symdiag}_r^{'}\ne\meansymb{\symdiag}_r$), and $\meanH_r^{'}\in \SymSecRankSpacetwoD$ is the deformed reference tensor, such that $\meanH_r^{'}\ne\meanH_r$. Clearly, the mean orientation $\meaneigvect_r$ of tensor $\meanH_r$ as defined in \feq{Eq:meanrot} is also preserved in the tensor $\meanH_r^{'}$ as shown in \feq{Eq:A26}.

To further elaborate the difference between tensors $\meanH_r$ and $\meanH_r^{'}$, let us 
reformulate the tensor $\meanH_r$ in the form:
\begin{equation}\label{Eq:meanCrotsplit}
\meanH_r = \meanH_r^{hyd}  +  \meanH_r^{dev}.
\end{equation}
Here $\meanH_r^{hyd}:={\text{tr}(\meanH_r)}/{2}$ and $\meanH_r^{dev}:=\meanH_r-\meanH_r^{hyd}$ are the hydrostatic and deviatoric components of tensor $\meanH_r$ respectively. Similarly, one can further rewrite tensor $\meanH_r^{'}$ as
\begin{equation}\label{Eq:meanCrotsplit1}
\meanH_r^{'}  = \meanH_r^{hyd}  +  \rho_2(\meanH_r^{dev}).
\end{equation}
It is clear that the shape of tensor $\meanH_r^{'}$ is altered by a factor of $\rho_2$ when compared to the tensor $\meanH_r$---seen on the deviatoric part in the above equation. 
Therefore, if the following condition
\begin{equation}\label{Eq:limE}
\lim\limits_{\rho_2\rightarrow1}  \mathbb{E}[\symtensor_r(\event_r)] = \meanH_r.
\end{equation}
is satisfied i.e. by normalizing the deviatoric part of tensor $\meanH_r^{'}$ by term $\rho_2$ in \feq{Eq:meanCrotsplit1}, 
one may say that the scaling aspect $\meansymb{\symdiag}_r$ of reference tensor $\meanH_r$ (from \feq{Eq:meanrot}) is also retained in tensor $\meanH_r^{'}$.

Analogous to \feqs{Eq:A25}{Eq:A26}, the Euclidean mean of stochastic tensor $\randrotscl(\event)\in\SymSecRankSpacetwoD$---with random scaling and orientation (see \feq{Eq:stomodrotscl})---may also be deduced into
\begin{equation}\label{Eq:meanrottilde2}
\mathbb{E}[\symtensor_{rs}(\event)] = \meaneigvect_r \meansymb{\symdiag}_s^{'} \meaneigvect_r^T = \meansymb{\symtensor}_{rs}^{'},
\end{equation}
in which $\meansymb{\symdiag}_s^{'}\in\mathbb{R}^{2\times 2}$ and $\meansymb{\symtensor}_{rs}^{'}\in \SymSecRankSpacetwoD$ represent the distorted versions of tensors $\meansymb{\symdiag}_s$ and $\meansymb{\symtensor}_{rs}$ respectively. Accordingly, one may re-represent the tensor $\meansymb{\symtensor}_{rs}^{'}$ as
\begin{equation}\label{Eq:meanCrotsplit2}
\meansymb{\symtensor}_{rs}^{'}  = \meansymb{\symtensor}_{rs}^{hyd}  +  \rho_2(\meansymb{\symtensor}_{rs}^{dev}).
\end{equation}
Here $\meansymb{\symtensor}_{rs}^{hyd}$ and $\meansymb{\symtensor}_{rs}^{dev}$ are the hydrostatic and deviatoric elements of reference tensor $\meansymb{\symtensor}_{rs}$. As shown in \feq{Eq:limE}, the change in shape of tensor $\meansymb{\symtensor}_{rs}^{'}$ when compared to tensor $\meansymb{\symtensor}_{rs}$ is normalized by satisfying the following condition: 
\begin{equation}\label{Eq:limE1}
\lim\limits_{\rho_2\rightarrow1}  \mathbb{E}[\symtensor_{rs}(\event)] = \meansymb{\symtensor}_{rs}.
\end{equation}

%In other words, one need not perform normalization by $\rho_2$.
%$\mathbb{E}[\symtensor_{rs}(\event)] = \meanCrotscl$
%is satisfied, without having to perform normalization by $\rho_2$.

%\begin{equation}
%\meanCrot^{'}  = \meanCrothyd  +  \rho_2(\meanCrotdev).
%\end{equation}

\subsection{Special case}

A special case emerges when the random tensor $\symtensor_{rs}(\event)$---from \feq{Eq:stomodrotscl}---is modelled, such that, the reference tensor $\meansymb{\symtensor}_{rs}$ in \feq{Eq:meanrotscl} particularly belongs to the isotropic symmetry, for instance:
\begin{equation}
\meansymb{\symtensor}_{rs} =
\begin{bmatrix}
\Crsoneone & 0  \\ 0 & \Crsoneone
\end{bmatrix},
\end{equation}
and the realizations 
% $\tilde{\symtensor}_{rs}(\event) = \symtensor_{rs}(\event)- \meansymb{\symtensor}_{rs}$
belong to a lower order of material symmetry (case of varying symmetry), along with random orientations. In such a scenario, the Euclidean mean of random tensor $\symtensor_{rs}(\event)$ naturally converges to mean $\meansymb{\symtensor}_{rs}$ and not to distorted mean $\meansymb{\symtensor}_{rs}^{'}$ i.e.
\begin{equation}
\mathbb{E}[\symtensor_{rs}(\event)] = \meaneigvect_r  \meanY_s  \meaneigvect_r^T =
\meansymb{\symtensor}_{rs}.
\end{equation}

%In particular, a special case emerges when the random tensor $\randrotscl(\event)$---from \feq{Eq:stomodrotscl}---is modelled, such that $\meansymb{\symdiag}_s$ in \feq{Eq:meanrotscl} is a scalar matrix i.e. all eigenvalues $\meaneigvalele_s, i=\left\lbrace 1,2\right\rbrace$ are equal. In such a scenario, the Euclidean mean of $\randrotscl(\event)$ converges naturally to $\meanCrotscl$ and not to $\meanCrotscl^{'}$. 

%\begin{equation}\label{Eq:meanrotscl}
%\meanCrotscl = \meaneigvect_r \ \meansymb{\symdiag}_s \ \meaneigvect_r^T.
%\end{equation}

%\begin{equation}\label{Eq:stomodrotscl1}
%\randrotscl(\event) = \rotmat(\rotangle(\event_r)) \ \meaneigvect_r \eigvalscl(\event_s) \meaneigvect_r^T \rotmat(\rotangle(\event_r))^T.
%\end{equation}
